# Supplementary material for: Upstream flow geometries can be uniquely learnt from single-point turbulence signatures
Source: arXiv:2412.10630 source file (2024-12-14)
Supplement: Supplementary file 1 [file arXiv_pdf_PNAS_SI.pdf]

## Supporting Information Text

Title: **Upstream flow geometries can be uniquely learnt from single-point turbulence signatures**
Authors: **Mukesh Karunanethy, Raghunathan Rengaswamy and Mahesh V Panchagnula**
Corresponding author e-mail: **Mahesh V Panchagnula: mvp@iitm.ac.in**

## Materials

**Experimental setup.** Figure S1 (page 6) shows a schematic of the experimental setup employed for time series measurements behind orifice plates inside a circular pipe. The setup consists of a mass-flow rate controller, a settling chamber, a long pipe with a provision to replace orifice plates, a hot wire anemometer and a data acquisition system (DAQ). 25 different orifice geometries were tested in the setup. All the orifices used for this study have been listed in table S8 (page 15). The cross-sectional area of the orifice opening was maintained the same for all geometries. The mass flow rate in the system was controlled using an Alicat Scientific® MCR-500SLPM-TFT/5M mass flow controller, which has a control range of 0.05 to 500$slpm$. This device helps maintain a fixed Reynolds number ($Re$) in the system. The Reynolds number was calculated based on the formula $Re = \rho VD/\mu$, where $\rho$ is the density of air ($1.223 kg/m^3$), $D$ is the diameter of a circular orifice ($26.8 \times 10^{-3} m$) of equivalent area, $V$ is the measured velocity at the orifice constriction, and $\mu$ is the dynamic viscosity of air at $25°$C ($1.85 \times 10^{-5} kg/ms$). Air through the mass flow controller enters a circular settling chamber of diameter $0.6m$. The settling chamber acts as a flow equalisation chamber that alleviates the fluctuations that might exist upstream of the chamber, such as any unsteady fluctuations from the mass flow controller or any valves upstream.

Air from the settling chamber enters a $300mm$ long circular pipe (Pipe 1 in figure S1 (page 6)) with an inner diameter of $50.8mm$ and an outer diameter of $60mm$. This pipe is long enough for the flow to be fully developed. A $2mm$ thick orifice plate is placed towards the end of this pipe, and another pipe of length $115mm$ (Pipe 2 in figure S1 (page 6)) was assembled after the orifice plate. A circular collar/coupler was utilised to seal and hold pipe 1, pipe 2, as well as the orifice plate together. The pipes and the coupler were made of rigid Polyvinyl chloride (PVC), and the orifice plates were cut out from a 304 stainless steel sheet (SS304) of $2mm$ thickness. Flow measurements were made downstream of the orifice plate (within pipe 2) using a Dantec Dynamics® 55R01 hot film probe. It consisted of a $1.25mm$ long, $70\mu m$ diameter nickel fibre film with $0.5\mu m$ quartz coating, which acts as the sensor. A Dantec Dynamics MiniCTA® 54T42 module housed the CT-HWA's signal processing and output for these measurements. The data logging was performed using a National Instruments® NI USB-6356 Multifunction DAQ connected to a computer. At a chosen cross-section, hot wire measurements were made at nine different locations, labelled as 'A', 'B', 'C', 'D', 'E', 'F', 'G', 'H' and 'I', as shown in the left-bottom of figure S1 (page 6). The spacing between consecutive probing points is $10mm$, both in $x$ and $y$ directions. A Halmarc® traverse system was utilised to precisely control the position of the probing point in $(x, y, z)$ directions.

**Dataset.** The experimental dataset collected for the orifice identification experiment is presented in table S1 (page 8). This tabulated data acts as a reference to all the experimental scenarios considered for this study. It represents a systematic examination of flow characteristics with different orifice geometries, sampling duration, and probing configurations. All the measurements were made at a consistent sampling rate of $10kHz$. Let us discuss the dataset provided row-wise. Row 1 shows 5 second signals recorded at the three different locations downstream of a circular orifice plate. These measurements were made along the centerline of the pipe. This set of measurements were performed to calibrate the system for flow rate and velocity. The mass flow rate was varied from $0slpm$ to $500slpm$ in steps of $50slpm$ and velocity was measured using the hot film probe. The measurements at location $1mm$ were utilised to get the calibration fit and, in turn, obtain the Reynolds number for each setting. Data from rows 2 and 3 were utilised to construct the velocity profiles previously discussed in the main manuscript. Data from rows 4 and 5 were utilized to study the sensitivity of the hot film probe to the flow conditions. Centerline velocity from a location immediately behind the plate to $22mm$ was profiled on two different days for this purpose. If there is a drift in the calibration curve after a day of probe usage, the profile will show a shift since all the flow conditions are maintained. Data from row 6, recorded for circle-, square- and equilateral triangle-shaped orifices were used to study the effect of flow rate on the performance of the algorithms. The remaining datasets in this table are 9-point measurements (locations 'A'−'I'). Data from rows 7 and 8 are for square- and circle-shaped orifices, the second one being the test data for the model trained on the first data. Row 8 also contains data from three different distances downstream of the plate, i.e., at $0.6D$, at $1.9D$ and at $4.2D$ distances behind the plate. Row 9 contains the data for all 25 geometries listed in table S8 (page 15). The measurements were made at $0.6D$ distance downstream of the plate, and the flow was maintained at $300slpm$. Five signals were recorded at each of the 9 locations. Note that the alignment of the system (position of the hot film probe with respect to the pipe setup) was maintained unchanged throughout these measurements for the 25 geometries. Test data were recorded from randomly chosen orifice plates to test the models built based on the dataset from row 9, such as data from rows 10 and 11. Data from rows 13 and 14 were used to understand the performance of the model build for square- and circle-shaped orifices. Time signals from behind the edges of the orifice and $5mm$ away from these edges would help us understand whether the presence of an edge in front of the probe affects the features learned by the models. The remaining data from rows 15 to 21 are test datasets to test the robustness of the model to system alignment. The model tested here was built using the data from square-, circle- and equilateral triangle-shaped orifices at $300slpm$. The system was shuffled physically, i.e., the alignment was removed and re-aligned four times for this study. All the test data includes 2 samples from all 9 locations. In this study, the 5 signals recorded for the model training will ensure the reproducibility of the time series, and the 2 test signals recorded after

realignment will help us study the repeatability of the system and the model. Three different CTAs and two different hot film probes, as listed in table S2 (page 9), were used for the repeatability study.

## Methods: Preprocessing steps

**Time series segmentation and normalization.** Segmentation is a common practice in time series analysis to divide a signal into smaller sub-sequences. This is particularly useful when dealing with non-stationary time series or when there are limited samples available for training machine learning models. By segmenting the time series based on certain statistical measures, it is possible to generate a larger number of representative samples for model training and testing.

The segmentation process is discussed below. Each of the time series (instantaneous voltage response) was recorded for $45s$ by sampling at a frequency of $10kHz$. This gives us a sufficiently resolved long series to perform segmentation without losing any significant information on the flow physics. Each time signal was divided into 179 overlapping segments using a window size equal to 1/90th the length of the signal and a sliding width of half the window size. Five signals were recorded at each of the 9 locations for each orifice geometry in the study. Out of the 5 signals, 4 were used for model training and the remaining 1 signal was used for model testing. The total number of representative samples thus obtained per location after segmentation is 895, with 5000 data points each.

Each time signal was normalized before feature extraction, ensuring that the time series were comparable across different realizations. This normalization process made the signals independent of the specific sensor used for measurement, as the extracted features depend only on the temporal correlation structure of the series, not on the raw data values. This approach can be described as *sensor-agnostic* (1). Whether the time series signal is obtained using a hot-wire/film probe or a laser-based technique, the algorithm's performance remains unaffected, provided there are sufficient data points to accurately capture the temporal structure of the flow. This allows us to develop an algorithm that relies on features invariant to the absolute values of the time series. To account for non-stationarity and variability within the data, z-score normalization is applied before feature extraction. The time series data was standardized by subtracting the mean and dividing by its standard deviation. This process ensures that each time series is centered around a mean of zero and has a standard deviation of one. Standardization helps mitigate the effects of varying breathing intensities and patterns, making the time series more comparable across different instances. It ensures that the features extracted from the time series are not influenced by changes in the overall magnitude of the data.

**Time series feature extraction.** An automated time series feature extraction algorithm named *tsfresh* (Time Series FeatuRe Extraction on the basis of Scalable Hypothesis tests) developed by Christ et al. (2) was utilised. This tool generates over 700 time series features using 63 different time series characterization methods. The following discussion pertains to preparing the dataset for model training and algorithm testing.

Features extracted from all available time series are concatenated and passed through a low-variance filter. This was done to remove those feature columns with a variance value below a given threshold, which in our case was 1%. The rationale behind applying this low-variance filter was to eliminate features that exhibit very little variation across instances. Such low-variance features may not provide useful insights for classification tasks. Furthermore, highly correlated features were removed from the feature set. A correlation threshold of 80% was chosen for this purpose. Removing features by these techniques reduces the dimensionality, simplifies the model, and potentially improves model performance by focusing on more informative features. All features that were derived from the absolute values of the time series, such as maximum/minimum values, quantile information, etc., were disregarded.

**Classifier models.** The classification problem can be formulated in two setups: $(i)$ class binarization approach and $(ii)$ Multi-class classifier approach. The former approach involves training ${}^{n}C_2$ binary classifier models, where $n$ is the total number of orifices. A library of all ${}^{n}C_2$ binary classifiers is termed a 'model library' in this manuscript. The latter approach involves training a single classifier model which classifies 25 orifices.

The random forest algorithm developed by Breiman (3) was employed in the process of training both binary and multi-class classifiers, utilizing a comprehensive hyperparameter tuning strategy, as detailed in Table S3 (page 10). The hyperparameters were carefully selected to ensure optimal model performance across various scenarios. The search space included the number of trees in the forest varying between 10 and 150, the criterion for measuring the quality of a split - the Gini impurity and entropy. Other tunable parameters, such as the number of features considered at every split, the maximum depth of the tree, and the method for selecting samples for training each tree, were also adjusted within defined ranges.

The tuning process employed a Bayesian Search Cross-Validation technique, which optimizes the model by searching across a pre-defined grid of hyperparameters. Specifically, the Bayesian Search was performed over 12 iterations, evaluating 12 models per iteration using 3-fold cross-validation. The scoring metric used was the micro-averaged F1 score, which balances the trade-off between precision and recall across all classes. Identical parameters and cross-validation schemes were applied for both binary and multi-class classifiers to ensure consistency in model training and to allow for a direct comparison of performance metrics. This approach ensured that the final models were robust and generalize well to unseen data.

## Methods: Orifice confirmation and identification algorithms

**Class binarization approach.** The orifice confirmation algorithm is employed to confirm the identity of an orifice based on a set of models previously trained on pairs of orifices' feature data. The algorithm presented (refer algorithm S1 (page 22)) operates

in two main stages: generating confirmations based on model predictions and making a final confirmation decision. The process begins by selecting models from a library that correspond to a given orifice. These models are then applied on the test data, and each model generates a predicted orifice ID. If the predicted ID matches the orifice in question, a confirmation counter will be incremented. The total number of confirmations is then compared to a predefined threshold, which is set to half the total number of orifices. If the confirmations exceed this threshold, the algorithm confirms the orifice's identity; otherwise, it does not confirm it.

The orifice identification algorithm presented (refer algorithm S2 (page 22)) extends the confirmation algorithm by focusing on determining the most likely identity of an orifice based on model predictions. This process involves two main stages: generating confirmation vectors and making a final identification decision. First, the algorithm iterates over all possible orifice identities, applying the confirmation algorithm to each one using the given test data and model library. The result is a confirmation vector $V_i$ for 'Orifice $i$', where each entry represents the number of model confirmations for a particular orifice ID. The algorithm then identifies the orifice that has received the highest number of confirmations across all models by selecting the maximum value in the confirmation vector. This orifice ID with the majority vote is returned as the identified orifice. This approach ensures a robust identification by leveraging the collective agreement among multiple predictive models. It is to be noted that when more than one confirmation trial results in the maximum prediction value, the algorithm does not identify an orifice.

**Multi-class classifier approach.** The latter approach utilises a multi-class random forest classifier model to classify 25 orifices. The model is applied to a given test data; it makes predictions on all the data points within the test data. The model assigns each data point a label/identity. The classifier's output can be interpreted as the model prediction probability, which is a vector denoted by $\Phi_i$, for 'Orifice $i$'. This vector's elements $a_1, a_2, \ldots, a_n$ represent the probability corresponding to each class label ($n$ is the total number of orifices). The orifice confirmation was then performed by setting a threshold for the probability. Here, a threshold of 50% was set for defining the minimum confidence of confirmation. This means that if the probability corresponding to the 'Orifice $i$' is greater than 0.5, the algorithm confirms the orifice's identity; otherwise, it does not confirm it.

The orifice identification algorithm focuses on identifying the orifice in the absence of prior knowledge. As observed from algorithm S4, the output of the random forest model was a prediction probability vector, $\Phi_i$, of size $(1, n)$. The identified orifice from this algorithm will then be the orifice corresponding to the maximum probability in the vector $\Phi_i$. If multiple classes have the same maximum probability, the algorithm does not identify a unique orifice. For the rest of the manuscript, we will only present orifice shape identification results since identification demands that the algorithm *identify* the orifice with no prior information.

The multi-class classifier approach generally scales more efficiently than the class binarization approach, especially for large numbers of orifices ($n$), because the multi-class random forest avoids running a separate binary classifier for each pair of orifices.

**Performance metrics.** The following are performance metrics (expressed in percentages) to evaluate the orifice geometry confirmation and identification algorithm:

1. True confirmation rate ($TCR$), which is a ratio of the confirmed geometries and total number of geometries as shown in equation 1.
$$TCR = \frac{c}{n} \times 100 \quad [1]$$
Here, $c$ and $u$ are the number of confirmed and unconfirmed orifice geometries, respectively. $u = 0$ when $TCR$ is 100%. $n$ is the total number of orifice geometries.

2. Accuracy ($A$), which quantifies the percentage of correctly identified orifice geometries out of all the orifices ($n$), demonstrating the algorithm's overall performance in correctly classifying orifice geometries.
$$A = \frac{t}{n} \times 100 \quad [2]$$
Here, $t$ is the value of true positives, i.e., the number of orifices that were identified correctly.

3. Precision ($P$) or Positive Predictive Value (PPV), which quantifies the accuracy of positive predictions, indicating the proportion of correctly identified orifice geometries among all the identified ones. This will offer insights into the algorithm's ability to avoid false positives.
$$P = \frac{t}{t+f} \times 100 \quad [3]$$
Here, $f$ is the value of false positives, i.e., the number of orifices that were identified incorrectly; and, $h$ is the number of orifices the algorithm was unable to identify.

## Results

The overall outcomes from the class binarization approach can be visualised using the identification matrix ($\mathbf{A}$). Figure S2 (page 7) shows an example of an identification matrix generated by running the orifice identification algorithm on all the $n = 25$ available orifice geometries. Matrix $\mathbf{A}$ can be seen as a stack of vectors, each with $n$ confirmation trials (refer algorithm S2

(page 22)). This approach utilised majority voting to identify an orifice geometry. The values in cells of each row represent a tested orifice identity, while each column represents one of the orifice identities for which a confirmation trial was performed.

Ideally, the identification matrix $\mathbf{A}$ from figure S2 (page 7) should contain non-zero model predictions only on the diagonal elements. Since the class binarization approach allows for prediction from all the models, this outcome with off-diagonal values, as shown in figure S2 (page 7), cannot be avoided. However, it is observed that diagonal elements are the maximum values in each row. In order to achieve a diagonal matrix, a runoff voting can be performed. Runoff voting, also known as a two-round system, is a popular method used in political elections. It is a voting method to elect a single winner from a field of more than two candidates (4). In the initial round of voting, voters cast their votes for their preferred candidates. If one candidate receives an outright majority (more than 50% of the votes), that candidate is declared the winner, and the process ends. If no candidate receives a majority in the first round, the two candidates with the highest number of votes proceed to a second round, which is referred to as a runoff. In the runoff round, voters are asked to vote again, typically for only one of the two remaining candidates. The candidate who receives the highest number of votes in the runoff is declared the winner.

This technique can be adopted in the identification algorithm. Initially, when a test orifice's data is given as input, the algorithm performs $n$ confirmation trials. It produces the vector $V$ as shown in algorithm S2 (page 22). This vector effectively contains votes or model predictions corresponding to every orifice geometry in the database. This is analogous to the initial round of voting. The total number of model predictions equals ${}^{25}C_2 = 300$. In the identification matrix, $\mathbf{A}$ shown in figure S2 (page 7), row (orifice ID) 0 has a maximum of 24 corresponding to column 0 and a second maximum of 23 corresponding to orifice ID = 5, which are around 8% of the total predictions/votes. This results in two trial orifices with the highest number of predictions proceeding to the runoff. Here, the runoff can be performed by testing only the model trained using orifice IDs 0 and 5. This would result in a modified identification matrix, $\bar{\mathbf{A}}$, which effectively is an identity matrix.

A better way to achieve a near-to-ideal case of an identity matrix is by using the single classifier approach as the identification algorithm. The results pertaining to this approach are discussed in the main manuscript.

**Repeatability and robustness to alignment.** A plausible way to ensure repeatability was by repeating the experiments and measuring test datasets for multiple system alignments. For simplicity, square, circle and equilateral triangle were the geometries chosen for this repeatability study. In each trial of alignment, the traverse mechanism was removed from its alignment, the orifice plate was removed and placed back, and the whole system was realigned. Initially, a 3−class random forest classifier model was trained using the data from system alignment #0. This dataset included five recorded signals, out of which four were used for model training and one signal was used for model testing. Thirty models were trained by shuffling the training and test feature set. Test data (2 signals of $45s$) were then recorded for four different alignments later, each for square-, circle- and equilateral triangle-shaped orifices and an additional randomly chosen orifice. The model prediction accuracy for the test data corresponding to the three geometries was computed and listed in table S4 (page 11). This ensures the repeatability of the results and robustness of the model to system alignment. The first column shows the alignment number, the constant temperature anemometer (CTA) circuit/module, and the hot film probe used for each alignment. The model numbers of these units were listed in table S2 (page 9). Given an alignment's test data, the output from the model would be the probabilities corresponding to each of the three geometries. The predicted geometries were sorted/ranked based on these probabilities, with Rank-1 denoting the highest probability.

Table S4 (page 11) displays the overall values of model prediction accuracy and the prediction probabilities (within square brackets), which can be seen as average model confidence. For square, circle and equilateral triangle geometries, the model predictions are shown for Rank-1 and Rank-2. For the randomly chosen geometries, the model prediction is compared to see how the model mispredicts them as square, circle or equilateral triangle. Let us discuss how the models identify these orifice geometries. For instance, in alignment #0, where the CTA-1 and Probe-1 were utilized, the model achieved 100% prediction accuracy for square, circle, and equilateral triangle geometries with 100% confidence. The results from this case can be considered a baseline for comparison since the training and test data were measured with the same alignment. However, we can observe from alignments #1, #2, #3, and #4 with CTA-1 and Probe-1, where minor changes in alignments could have been introduced due to handling errors, slight variations in prediction accuracies were observed. Despite these variations, the model maintains a high level of accuracy for all three geometries, except for square in alignment #1, where it was ranked highest only 88.9% of the time. These observations suggest a certain degree of tolerance to alignment imperfections between the training and test datasets.

For alignment #3, two different CTAs were also tested with Probe-1: CTA-2 and CTA-3 in order to ascertain that there is no measurement system artifact. CTA-3 produced similar performance to CTA-1, with a slight drop in the prediction accuracy only for the circular orifice. Whereas, the data measured with CTA-2 produced poor results for the square geometry. However, the model predicted the circle and equilateral triangle correctly, even for CTA-2. It was hindering the ability of the classifier to predict a square. A similar observation was made in alignment #4 as well when CTA-2 was used. This observation remained anomalous as the reason was not identified. For the alignment #4, when Probe-2 was used along with CTA-1, the model achieved 100% prediction accuracy for all three geometries.

**Effect of flow rates.** All the results discussed so far were based on the analyses performed with a system mass flow rate of $300 slpm$, which produces a Reynolds number of $2.37 \times 10^4$ based on the orifice opening. Understanding the performance of the binary classifier for various Reynolds numbers ($Re$) becomes interesting at this point. To understand this, 9-point ('A'−'I') time series measurements were made for square- and circle-shaped orifices at $z = 0.6D$ for different system $Re$. The $Re$ corresponding to each of the mass flow rates considered are listed in table S5 (page 12).

Table S6 (page 13) shows the model prediction accuracy corresponding to different combinations of test data and classifiers, each considered for various $Re$. Each cell in this table represented the accuracy value in the following format: '*median* (*interquartile range*)'. The 'Model' column presents the prediction accuracies for random forest models trained on the datasets corresponding to 4 different $Re$. The 'Test data' column shows the test dataset corresponding to each $Re$. The results presented are based on 50 realisations for training-test shuffling. These metrics were chosen to describe the accuracy values due to the skewed distribution of the test scores. The median and interquartile range (IQR) represent the central tendency and variability, respectively, of the accuracy values.

By examining the results from table S6 (page 13), it is evident that the model generally achieves high accuracy across the flow rates, with median accuracy values consistently exceeding 95% for most test data and $Re$ combinations. Also, when the test data and the trained model were from the same $Re$, the model achieved 100% accuracy consistently as expected. This outlines the robustness of the random forest classifier in accurately classifying circle and square orifices, irrespective of the system $Re$. Moreover, analyzing the IQR values provides insight into the variability of the accuracy scores. For instance, in cases where the IQR is relatively small, such as for test data and models corresponding to the $Re$ between $2.37 \times 10^4$ to $3.17 \times 10^4$, the models exhibit high consistency in their performance. This means that accuracy scores were tightly clustered around the median value. This also suggests a high confidence level in the model's predictions within this range of $Re$. The only case with a slightly lower accuracy in this range is for the prediction of test data from $Re = 2.37 \times 10^4$ predicted by a model built on $Re = 3.17 \times 10^4$ data, showing an accuracy of 86% with a spread of 6.8%. Conversely, the test data associated with $Re = 1.97 \times 10^4$ showed interesting results. It showed increased variability in accuracy scores for models built on higher $Re$, with the lowest accuracy observed being 78% against a model trained on $Re = 3.17 \times 10^4$ data. The model trained on $Re = 1.97 \times 10^4$ data also showed a small drop in accuracy when tested with the rest of the test datasets. In conclusion, it is best to train the model for a Reynolds number of $2.37 \times 10^4$ or $2.77 \times 10^4$, which can be used across a wide range of $Re$.

Overall, these variabilities observed across the $Re$ considered here may stem from the influence of the turbulence characteristics of the flow, which could be specific to each mass flow rate setting. Any difference in the time series features due to variations in flow characteristics could introduce additional complexity in the classification. The models generally get optimised for these features observed in the training dataset. For the models to make perfect predictions across different flow conditions, they must be further refined or trained by accommodating the variations associated with the diverse operating conditions.

**Performance at varying distances downstream.** All the analyses discussed so far were based on the time series measurements at a distance $z = 0.6D$ behind the orifice plate. Recalling the velocity and turbulence intensity ($TI$) profiles in the main manuscript, we observed that with increasing distance downstream of the orifice plate, the $TI$ increases on average, implying the growth of the level of turbulence. The objective was to determine how much information about the orifice geometry is preserved in the downstream flow. To understand this, 9-point ('A'−'I') time series measurements were made for square- and circle-shaped orifices at three different distances downstream: (*i*) at $z = 0.6D$, (*ii*) at $z = 1.9D$, and (*iii*) at $z = 4.2D$. Table S7 (page 14) presents the test data accuracies of binary random forest classifiers built at these three distances. The test accuracy presented here is defined as the percentage of test data points correctly classified. A higher accuracy would mean better classifiability between circle and square geometries, and a low value of test accuracy would mean that the square and circle are not classifiable. The accuracy values are represented in the following format: '*mean* $\pm 2\times$ *standard deviation*'. These results are based on 20 realisations of train-test shuffling. At distance $z = 0.6D$, the geometries are classifiable with nearly 100% accuracy at the probing points near the edges ('B', 'D', 'G', and 'H'). At the points near the wall ('A', 'E', 'F', and 'I'), the accuracy achieved is roughly between 65% to 85%, indicating a moderate classifiability. The asymmetry in the accuracy (between the left-right and top-bottom sides in the flow field) is observed due to minute variations in the alignment along the $x$-$y$ plane. At the centre (point 'C'), the accuracy is around 73%, which could be considered as moderate classifiability. Now, looking at distance $z = 1.9D$, the range of accuracy at the points near the wall remains roughly the same, but the accuracies achieved near the edges were observed to decrease by approximately between 20% to 35%. At point 'C', the accuracy decreased to around 66%, which could again be inferred as moderate classifiability. Furthermore, at a distance $z = 4.2D$, there was a significant drop in accuracy at all locations except for point 'C', where it remained roughly the same. The accuracies near the edges were observed to further decrease by around 15% to 30% from that at distance $z = 1.9D$. The accuracy had decreased to nearly 60% at the points near the wall. The results from the distance $z = 4.2D$ can be interpreted as low classifiability compared to the other distances upstream.

Now, when data from all the 9 locations ('A'−'I') were combined, the overall accuracy still seemed to decrease with an increase in distance downstream of the orifice plate. The accuracy was observed to be around 100% at $z = 0.6D$ and 97% at $z = 1.9D$ followed by 78% at $z = 4.2D$. The observations from this study imply that the information on the geometry of an orifice is partially preserved in the flow field downstream, with its strength remaining high until a distance roughly equal to two orifice diameters. As expected, this information would be gradually lost beyond this distance, owing to the nature of a fully developed jet.

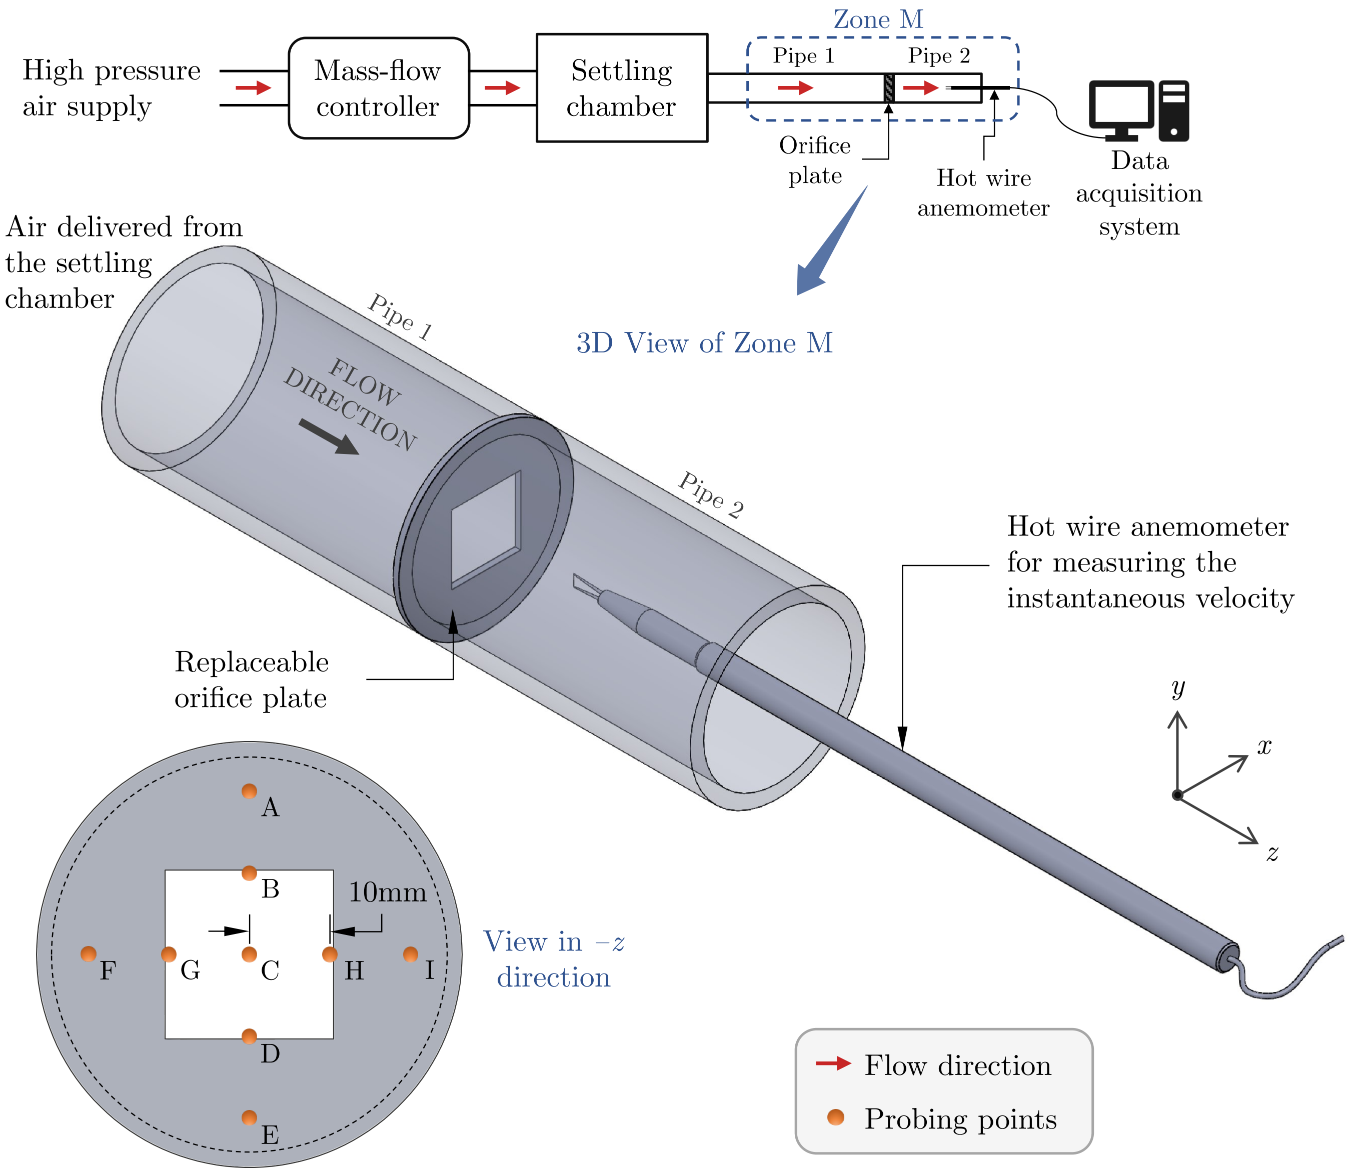


**Fig. S1.** Depiction of the experimental setup for time series measurements. It consists of a mass-flow controller, a settling chamber, a long pipe with a provision to replace orifice plates, a hot wire anemometer and a data acquisition system. The hot wire probe was traversed in $x$, $y$ and $z$ directions for measurements. *Bottom left*: The assigned sampling points were $9$ locations labelled 'A', 'B', 'C', 'D', 'E', 'F', 'G', 'H' and 'I'. The probing points were spaced horizontally and vertically with a $10mm$ distance. The area within the black dotted lines is exposed to the flow.

Trial orifice identity →

↓ True orifice identity

| | 0 | 1 | 2 | 3 | 4 | 5 | 6 | 7 | 8 | 9 | 10 | 11 | 12 | 13 | 14 | 15 | 16 | 17 | 18 | 19 | 20 | 21 | 22 | 23 | 24 | |
|---|---|---|---|---|---|---|---|---|---|---|---|---|---|---|---|---|---|---|---|---|---|---|---|---|---|---|
| 0 | 24 | 18 | 19 | 12 | 19 | 23 | 13 | 6 | 8 | 9 | 22 | 0 | 11 | 11 | 9 | 19 | 7 | 4 | 8 | 9 | 2 | 16 | 15 | 7 | 9 | 0 |
| 1 | 4 | 24 | 15 | 20 | 4 | 1 | 19 | 10 | 2 | 4 | 10 | 10 | 11 | 17 | 8 | 4 | 22 | 14 | 7 | 16 | 19 | 20 | 3 | 13 | 23 | 1 |
| 2 | 5 | 12 | 24 | 19 | 2 | 1 | 16 | 8 | 4 | 5 | 9 | 10 | 23 | 20 | 5 | 3 | 17 | 14 | 10 | 22 | 14 | 20 | 4 | 17 | 16 | 2 |
| 3 | 5 | 13 | 18 | 24 | 3 | 2 | 15 | 9 | 4 | 3 | 9 | 10 | 14 | 21 | 9 | 3 | 22 | 19 | 8 | 20 | 18 | 12 | 1 | 17 | 21 | 3 |
| 4 | 20 | 15 | 10 | 14 | 24 | 20 | 11 | 13 | 0 | 1 | 19 | 8 | 8 | 4 | 18 | 23 | 14 | 5 | 2 | 13 | 4 | 11 | 22 | 8 | 13 | 4 |
| 5 | 23 | 11 | 17 | 10 | 20 | 24 | 16 | 5 | 9 | 14 | 22 | 0 | 11 | 11 | 12 | 18 | 6 | 4 | 6 | 9 | 2 | 13 | 20 | 6 | 11 | 5 |
| 6 | 8 | 18 | 19 | 22 | 0 | 7 | 24 | 7 | 2 | 4 | 9 | 9 | 12 | 21 | 4 | 2 | 17 | 14 | 10 | 19 | 13 | 23 | 4 | 15 | 17 | 6 |
| 7 | 3 | 17 | 14 | 15 | 1 | 1 | 6 | 24 | 9 | 11 | 3 | 23 | 18 | 8 | 20 | 7 | 20 | 11 | 12 | 11 | 16 | 13 | 3 | 15 | 19 | 7 |
| 8 | 9 | 7 | 14 | 12 | 2 | 9 | 8 | 16 | 24 | 23 | 14 | 13 | 18 | 18 | 21 | 0 | 7 | 14 | 22 | 5 | 13 | 8 | 1 | 14 | 8 | 8 |
| 9 | 8 | 9 | 17 | 11 | 1 | 7 | 7 | 16 | 23 | 24 | 14 | 13 | 18 | 17 | 20 | 0 | 10 | 13 | 22 | 4 | 16 | 10 | 2 | 7 | 11 | 9 |
| 10 | 23 | 19 | 17 | 11 | 15 | 22 | 13 | 3 | 5 | 9 | 24 | 0 | 6 | 9 | 5 | 19 | 16 | 5 | 4 | 8 | 10 | 15 | 18 | 7 | 17 | 10 |
| 11 | 1 | 11 | 13 | 16 | 4 | 0 | 11 | 18 | 6 | 4 | 2 | 24 | 22 | 13 | 16 | 7 | 17 | 21 | 8 | 13 | 21 | 10 | 5 | 20 | 17 | 11 |
| 12 | 5 | 10 | 23 | 18 | 1 | 5 | 16 | 9 | 4 | 3 | 8 | 13 | 24 | 21 | 5 | 3 | 15 | 20 | 10 | 15 | 18 | 17 | 3 | 21 | 13 | 12 |
| 13 | 8 | 12 | 18 | 23 | 1 | 5 | 17 | 4 | 7 | 6 | 10 | 8 | 19 | 24 | 4 | 1 | 15 | 22 | 11 | 14 | 20 | 16 | 1 | 21 | 13 | 13 |
| 14 | 12 | 7 | 7 | 9 | 9 | 6 | 1 | 22 | 18 | 10 | 4 | 23 | 11 | 7 | 24 | 9 | 12 | 17 | 19 | 11 | 16 | 4 | 8 | 17 | 17 | 14 |
| 15 | 15 | 10 | 12 | 9 | 22 | 17 | 6 | 16 | 0 | 1 | 15 | 16 | 16 | 3 | 21 | 24 | 14 | 8 | 2 | 10 | 10 | 6 | 23 | 12 | 12 | 15 |
| 16 | 4 | 15 | 19 | 21 | 2 | 1 | 15 | 10 | 1 | 4 | 7 | 11 | 13 | 12 | 9 | 4 | 24 | 15 | 8 | 20 | 21 | 19 | 5 | 17 | 23 | 16 |
| 17 | 5 | 12 | 15 | 22 | 3 | 2 | 14 | 8 | 4 | 4 | 7 | 12 | 17 | 21 | 9 | 3 | 19 | 24 | 9 | 17 | 20 | 12 | 1 | 23 | 17 | 17 |
| 18 | 6 | 8 | 18 | 14 | 2 | 4 | 12 | 12 | 23 | 22 | 6 | 6 | 20 | 20 | 18 | 0 | 10 | 16 | 24 | 8 | 15 | 13 | 1 | 13 | 9 | 18 |
| 19 | 4 | 13 | 22 | 23 | 3 | 2 | 17 | 9 | 4 | 4 | 8 | 10 | 16 | 15 | 8 | 3 | 20 | 16 | 8 | 24 | 14 | 15 | 3 | 18 | 21 | 19 |
| 20 | 3 | 12 | 14 | 19 | 2 | 1 | 14 | 9 | 3 | 3 | 9 | 11 | 17 | 19 | 8 | 4 | 21 | 23 | 8 | 14 | 24 | 16 | 5 | 20 | 21 | 20 |
| 21 | 6 | 20 | 20 | 16 | 2 | 1 | 23 | 8 | 2 | 4 | 10 | 9 | 18 | 17 | 5 | 3 | 21 | 13 | 10 | 14 | 17 | 24 | 6 | 12 | 19 | 21 |
| 22 | 20 | 10 | 17 | 7 | 21 | 20 | 9 | 9 | 0 | 1 | 21 | 9 | 16 | 6 | 14 | 23 | 14 | 4 | 3 | 5 | 10 | 17 | 24 | 8 | 12 | 22 |
| 23 | 4 | 13 | 17 | 22 | 2 | 3 | 14 | 9 | 4 | 4 | 7 | 11 | 18 | 19 | 9 | 3 | 16 | 23 | 8 | 18 | 20 | 12 | 2 | 24 | 18 | 23 |
| 24 | 2 | 17 | 19 | 21 | 4 | 1 | 15 | 9 | 2 | 5 | 8 | 10 | 13 | 12 | 9 | 4 | 23 | 14 | 8 | 20 | 21 | 18 | 4 | 17 | 24 | 24 |
| | 0 | 1 | 2 | 3 | 4 | 5 | 6 | 7 | 8 | 9 | 10 | 11 | 12 | 13 | 14 | 15 | 16 | 17 | 18 | 19 | 20 | 21 | 22 | 23 | 24 | |

**Fig. S2.** The identification matrix $(\mathbf{A})$ contains the votes or the sum of model predictions corresponding to each possible orifice identity. Each row represents a tested orifice identity, while each column represents one of the orifice identities for which a confirmation trial was performed. Since the model was trained for all $25$ geometries, and confirmation trials were performed for all those geometries, the shape of this matrix is $25 \times 25$. In each row, the highest and second-highest voted cells have been marked black and grey, respectively.

**Table S1. Tabulation of recorded hot film time signals for various cases involving the flow past orifice inside a circular pipe. All the measurements were made at a sampling rate of $10kHz$.**

| Sl. No. | Orifice geometry | Sampling duration | Probing points and number of samples | Distance downstream $(mm)$ | Flow-rate $(slpm)$ |
|---|---|---|---|---|---|
| 1 | Circle (Flow rate calibration - Axial measurements) | $5s$ | 1 point, 1 sample | 1, 6, 16 | 0 - 500 † |
| 2 | No orifice (Velocity profile) | $20s$ | 55 points, 1 sample each | – | 300 |
| 3 | Circle (Velocity profile) | $5s$, $20s$ | 52 points, 1 sample each | 17, 112 | 300 |
| 4 | Circle (Centerline velocity with distance) | $5s$ | 1 point, 1 sample | 0 - 22 * | 300 |
| 5 | Circle (Centerline velocity with distance) (Repeat) | $5s$ | 1 point, 1 sample | 0 - 22 * | 300 |
| 6 | Circle \| Square \| Triangle (Effect of flow rate) | $45s$ | 9 points, 5 samples each | 16 | 250 - 400 † |
| 7 | Circle \| Square | $45s$ | 9 points, 4 samples each | 17 | 300 |
| 8 | Circle \| Square (Repeat) | $45s$ | 9 points, 5 samples each | 17, 50.8, 112 | 300 |
| 9 | Geometries 1 to 25 (refer Table S8 for the list) | $45s$ | 9 points, 5 samples each | 16 | 300 |
| 10 | Square \| Six-pointed star (Test data) | $45s$ | 9 points, 2 samples each | 16 | 300 |
| 11 | Circle (Test data) | $45s$ | 9 points, 2 samples each | 16 | 300 |
| 12 | Circle \| Square \| Triangle \| Random (Align.1) | $45s$ | 9 points, 3 samples each | 16 | 300 |
| 13 | Circle \| Square (Edge data) | $45s$ | 4 edges, 5mm from edges, 5 samples each | 16 | 300 |
| 14 | Circle \| Square (Edge - Test data) | $45s$ | 4 edges, 5mm from edges, 2 samples each | 16 | 300 |
| 15 | Circle \| Square \| Triangle \| Random (Aligns.2,3) | $45s$ | 9 points, 2 samples each | 16 | 300 |
| 16 | Circle \| Square \| Triangle (Align.3; CTA-2,3) | $45s$ | 9 points, 2 samples each | 16 | 300 |
| 17 | Square (Align.3; CTA-2) | $45s$ | 9 points, 2 samples each | 16 | 300 |
| 18 | Circle \| Square \| Triangle (Align.4; CTA-2) | $45s$ | 9 points, 2 samples each | 16 | 300 |
| 19 | Circle \| Square \| Triangle (Flow rate - Test data) (Align.4) | $45s$ | 9 points, 2 samples each | 16 | 250 - 400 † |
| 20 | Circle \| Square \| Triangle (Align.4; Probe-2) | $45s$ | 9 points, 2 samples each | 16 | 300 |

Align. ≡ Alignment; * $1mm$ steps; † $50slpm$ steps.

**Table S2. List of constant temperature anemometers (CTA) and the hot film probes used for the orifice geometry identification experiments**

| Label | CTA/Probe |
|---|---|
| CTA-1 | Dantec Dynamics MiniCTA® $54\mathrm{T}42$ |
| CTA-2 | Dantec Dynamics Multichannel CTA® $54\mathrm{N}81$ (Channel-1) |
| CTA-3 | Dantec Dynamics MiniCTA® $54\mathrm{T}42$ |
| Probe-1 | Dantec Dynamics® $55\mathrm{R}01$ hot film |
| Probe-2 | Dantec Dynamics® $55\mathrm{R}01$ hot film |

**Table S3. A list of hyperparameters and their search space chosen for binary and multi-class classification**

| Hyperparameter | List of values |
|---|---|
| Tunable parameters for the Random Forest model | |
| Number of trees in random forest (n_estimators) | linspace(start = 10, stop = 150, num = 100) |
| The function to measure the quality of a split (criterion) | ['gini', 'entropy'] |
| Number of features to consider at every split (max_features) | ['log2', 'sqrt'] |
| Maximum number of levels in tree (max_depth) | linspace(2, 100, num = 20) + [None] |
| Minimum number of samples required to split a node (min_samples_split) | [2, 5, 10] |
| Minimum number of samples required at each leaf node (min_samples_leaf) | [1, 2, 4] |
| Method of selecting samples for training each tree (bootstrap) | [True, False] |
| Parameters specific to the optimization technique | |
| Optimization technique | Bayesian Search cross validation |
| Number of iterations (n_iter) | 12 |
| Scoring metric (scoring) | F1 score (f1_micro) |
| Number of models evaluated per iteration (n_points) | 12 |
| Number of cross-validation folds (cv) | 3 |

Parameters in typewriter font are from the Scikit-learn package (5) in Python®.

**Table S4. Model prediction accuracy on test geometries. The values are represented in the format '*accuracy* [*average model confidence*]'. CTA stands for Constant Temperature Anemometer.**

| Alignment | Square (S) | | Circle (C) | | Equilateral triangle (T) | |
|---|---|---|---|---|---|---|
| | Rank-1 (%) | Rank-2 (%) | Rank-1 (%) | Rank-2 (%) | Rank-1 (%) | Rank-2 (%) |
| #0 (CTA-1; Probe-1) | 100.0 [100.0] | 0.0 [−] | 100.0 [100.0] | 0.0 [−] | 100.0 [100.0] | 0.0 [−] |
| #1 (CTA-1; Probe-1) | 88.9 [64.5] | 11.1 [46.6] | 100.0 [100.0] | 0.0 [−] | 100.0 [100.0] | 0.0 [−] |
| #2 (CTA-1; Probe-1) | 100.0 [91.4] | 0.0 [−] | 100.0 [100.0] | 0.0 [−] | 100.0 [100.0] | 0.0 [−] |
| #3 (CTA-1; Probe-1) | 100.0 [98.8] | 0.0 [−] | 100.0 [100.0] | 0.0 [−] | 100.0 [100.0] | 0.0 [−] |
| #3 (CTA-2; Probe-1) | 0.0 [−]<br>0.0 [−] | 40.0 [1.6]<br>96.7 [11.3] | 100.0 [100.0] | 0.0 [−] | 100.0 [97.2] | 0.0 [−] |
| #3 (CTA-3; Probe-1) | 100.0 [99.1] | 0.0 [−] | 90.0 [72.2] | 10.0 [41.5] | 100.0 [100.0] | 0.0 [−] |
| #4 (CTA-1; Probe-1) | 100.0 [94.6] | 0.0 [−] | 100.0 [100.0] | 0.0 [−] | 100.0 [100.0] | 0.0 [−] |
| #4 (CTA-2; Probe-1) | 0.0 [−] | 3.3 [0.6] | 100.0 [100.0] | 0.0 [−] | 96.7 [93.9] | 3.3 [35.2] |
| #4 (CTA-1; Probe-2) | 100.0 [91.6] | 0.0 [−] | 100.0 [100.0] | 0.0 [−] | 100.0 [100.0] | 0.0 [−] |

**Table S5. Mass flow rates considered for the analyses and corresponding Reynolds numbers ($Re$). $Re$ was computed based on the measured velocity at the orifice constriction and diameter of the circular orifice**

| Mass flow rate ($slpm$) | Reynolds number |
|---|---|
| $250slpm$ | $1.97 \times 10^4$ |
| $300slpm$ | $2.37 \times 10^4$ |
| $350slpm$ | $2.77 \times 10^4$ |
| $400slpm$ | $3.17 \times 10^4$ |

**Table S6. Model prediction accuracies (*median* and IQR) for different test data and model combinations based on $Re$**

| Test data | Model | | | |
|---|---|---|---|---|
| | $1.97 \times 10^4$ | $2.37 \times 10^4$ | $2.77 \times 10^4$ | $3.17 \times 10^4$ |
| $1.97 \times 10^4$ | 100 (0) | 98 (1.8) | 94 (6.0) | 78 (12.6) |
| $2.37 \times 10^4$ | 99 (1.8) | 100 (0) | 100 (0) | 86 (6.8) |
| $2.77 \times 10^4$ | 96 (7.2) | 100 (0) | 100 (0) | 100 (0.2) |
| $3.17 \times 10^4$ | 97 (4.4) | 100 (0.2) | 100 (0) | 100 (0) |

**Table S7. Model prediction accuracies (median $\pm$ standard deviation) for classification of square and circular orifices for various distances downstream. The results are based on $20$ realisations of train-test shuffling**

| Location | Distance from orifice | | |
|---|---|---|---|
| | $z = 0.6D$ | $z = 1.9D$ | $z = 4.2D$ |
| A | $72 \pm 7.3$ | $67 \pm 5.8$ | $61 \pm 8.0$ |
| B | $98 \pm 1.0$ | $65 \pm 6.3$ | $52 \pm 5.4$ |
| C | $73 \pm 6.7$ | $66 \pm 7.9$ | $69 \pm 6.5$ |
| D | $97 \pm 3.2$ | $65 \pm 4.6$ | $51 \pm 6.6$ |
| E | $74 \pm 10.0$ | $78 \pm 5.7$ | $63 \pm 4.2$ |
| F | $64 \pm 8.4$ | $88 \pm 4.0$ | $59 \pm 5.8$ |
| G | $97 \pm 2.1$ | $79 \pm 5.8$ | $52 \pm 4.3$ |
| H | $100 \pm 0$ | $70 \pm 3.3$ | $52 \pm 5.5$ |
| I | $84 \pm 8.1$ | $85 \pm 5.0$ | $66 \pm 5.6$ |
| A−I | $\mathbf{100 \pm 0}$ | $\mathbf{97 \pm 1.5}$ | $\mathbf{78 \pm 4.5}$ |

Table S8. Orifice geometries which were studied. Each geometry is defined by a characteristic length, and these characteristic lengths are defined as a proportion of the diameter of the orifice plate, D. Note that this diameter is equal to the outer diameter of the plate, which was considered for manufacturing and mounting purposes.

| Label | Characteristic length of an orifice geometry | Area of the orifice | Relation with plate diameter |
|---|---|---|---|
| 01 | Circle 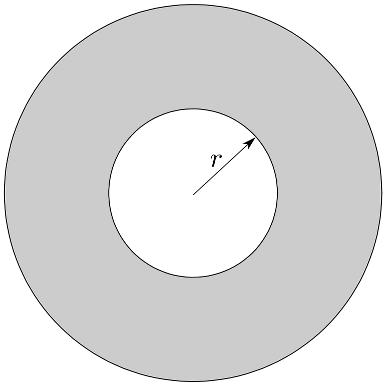  | $\pi r^2$ | $r = (0.223606)\mathbf{D}$ |
| 02 | Square 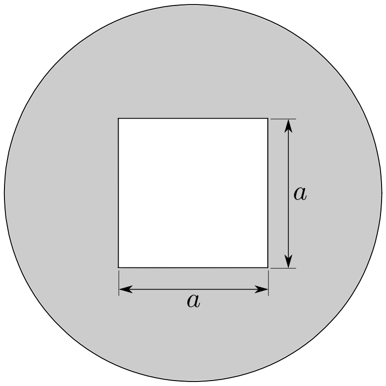  | $a^2$ | $a = (0.396332)\mathbf{D}$ |
| 03 | Ellipse 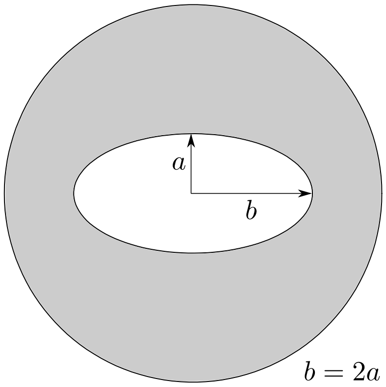  | $\pi ab$ | $a = (0.158113)\mathbf{D}$ |

*Continued on next page*

Table S8 – Orifice geometries which were studied (*Continued from previous page*)

| Label | Characteristic length of an orifice geometry | Area of the orifice | Relation with plate diameter |
|---|---|---|---|
| 04 | Equilateral triangle 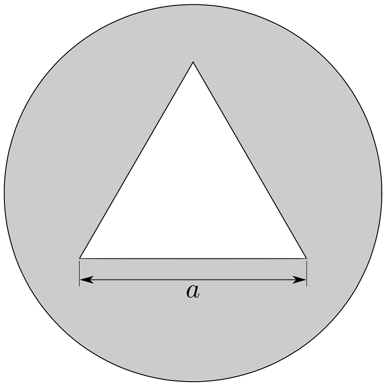  | $\frac{\sqrt{3}}{4}a^2$ | $a = (0.602295)\mathbf{D}$ |
| 05 | Isosceles triangle 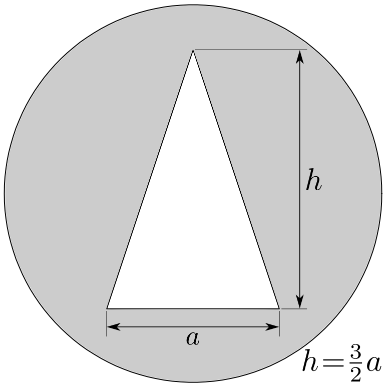  | $\frac{1}{2}ah$ | $a = (0.457645)\mathbf{D}$ |
| 06 | Acute-angled triangle 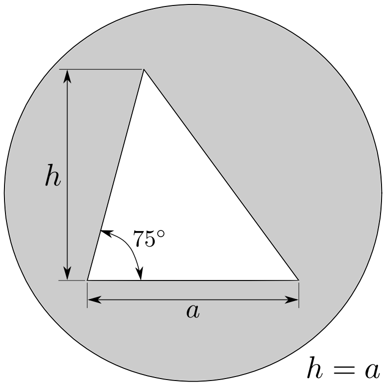  | $\frac{1}{2}ah$ | $a = (0.560499)\mathbf{D}$ |
| 07 | Obtuse-angled triangle 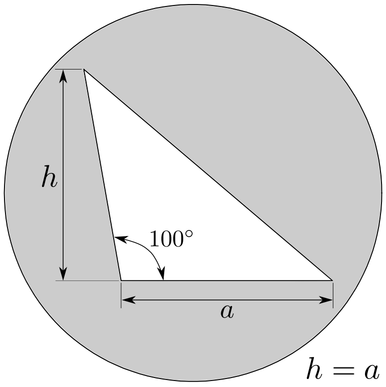  | $\frac{1}{2}ah$ | $a = (0.560499)\mathbf{D}$ |

*Continued on next page*

Table S8 – Orifice geometries which were studied (*Continued from previous page*)

| **Label** | **Characteristic length of an orifice geometry** | **Area of the orifice** | **Relation with plate diameter** |
|---|---|---|---|
| 08 | Right-angled triangle 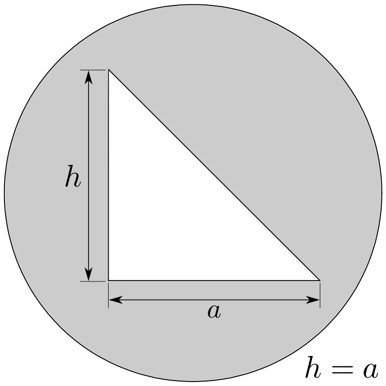  | $\frac{1}{2}ah$ | $a = (0.560499)\mathbf{D}$ |
| 09 | Rectangle 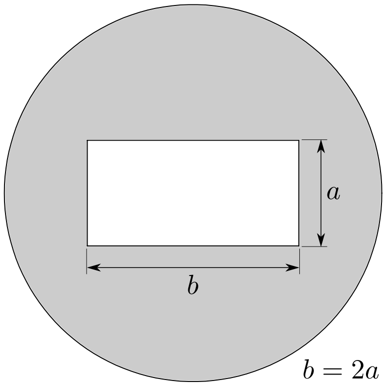  | $ab$ | $a = (0.280249)\mathbf{D}$ |
| 10 | Heart 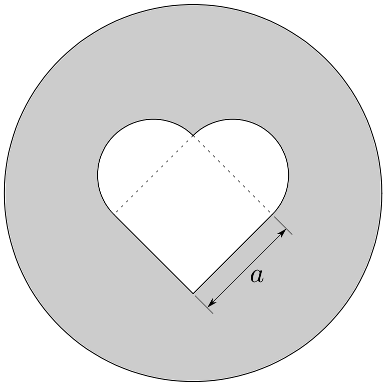  | $\left(1+\frac{\pi}{4}\right)a^2$ | $a = (0.296614)\mathbf{D}$ |
| 11 | Parallelogram 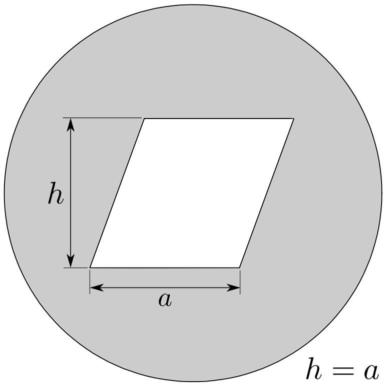  | $ah$ | $a = (0.396332)\mathbf{D}$ |

*Continued on next page*

Table S8 – Orifice geometries which were studied (*Continued from previous page*)

| **Label** | **Characteristic length of an orifice geometry** | **Area of the orifice** | **Relation with plate diameter** |
|---|---|---|---|
| 12 | Trapezium 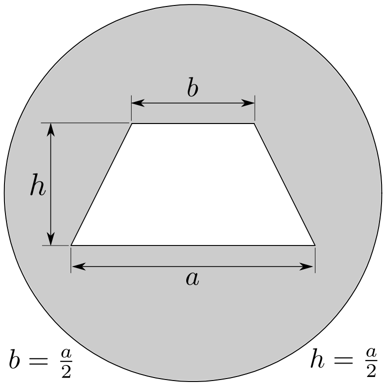  | $\frac{a+b}{2}h$ | $a = (0.647208)\mathbf{D}$ |
| 13 | Rhombus 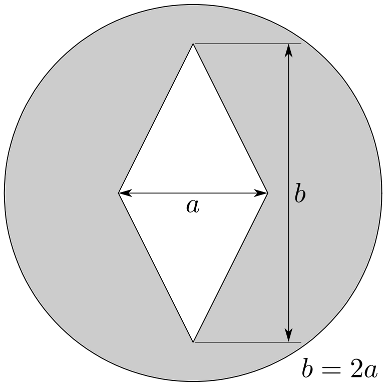  | $\frac{ab}{2}$ | $a = (0.396332)\mathbf{D}$ |
| 14 | Semi-circle 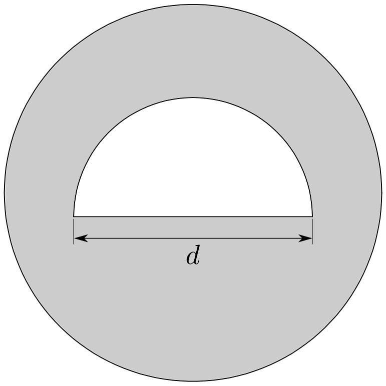  | $\frac{\pi d^2}{8}$ | $d = (0.632455)\mathbf{D}$ |
| 15 | Quadrant 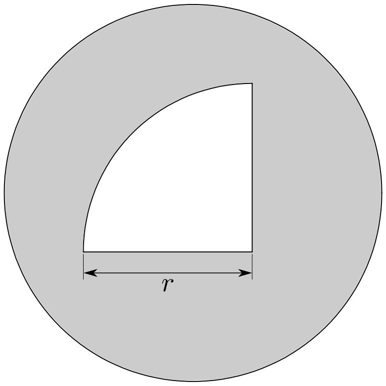  | $\frac{\pi r^2}{4}$ | $r = (0.447213)\mathbf{D}$ |

*Continued on next page*

Table S8 – Orifice geometries which were studied (*Continued from previous page*)

| **Label** | **Characteristic length of an orifice geometry** | **Area of the orifice** | **Relation with plate diameter** |
|---|---|---|---|
| 16 | Kite 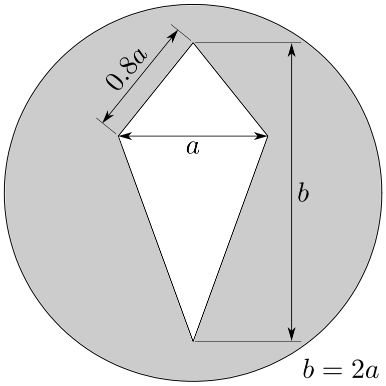  | $\frac{ab}{2}$ | $a = (0.396332)\mathbf{D}$ |
| 17 | Pentagon 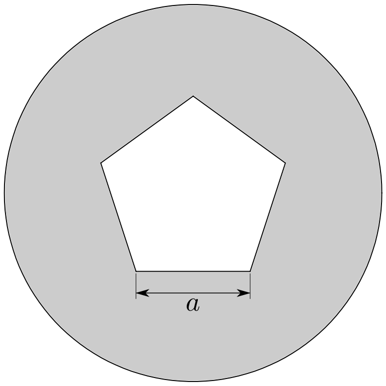  | $\frac{1}{4}\sqrt{5(5+2\sqrt{5})}a^2$ | $a = (0.302158)\mathbf{D}$ |
| 18 | Hexagon 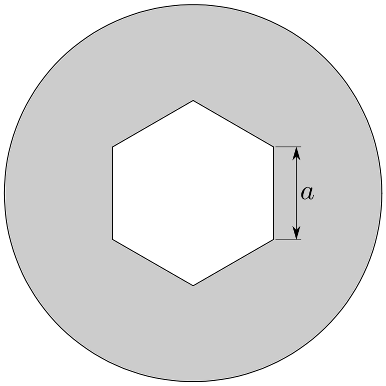  | $\frac{3\sqrt{3}}{2}a^2$ | $a = (0.245886)\mathbf{D}$ |
| 19 | Heptagon 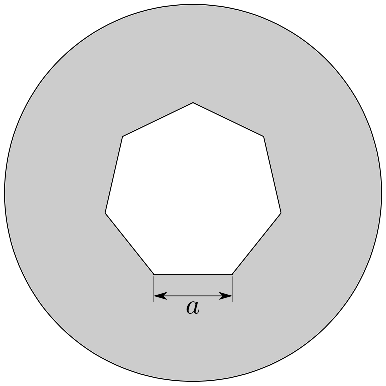  | $\frac{7}{4}a^2 \cot\left(\frac{\pi}{7}\right)$ | $a = (0.207908)\mathbf{D}$ |

*Continued on next page*

Table S8 – Orifice geometries which were studied (*Continued from previous page*)

| Label | Characteristic length of an orifice geometry | Area of the orifice | Relation with plate diameter |
|---|---|---|---|
| 20 | Octagon 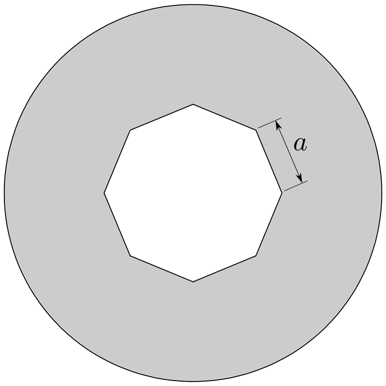  | $2\left(1+\sqrt{2}\right)a^2$ | $a = (0.180367)\mathbf{D}$ |
| 21 | Four-pointed star 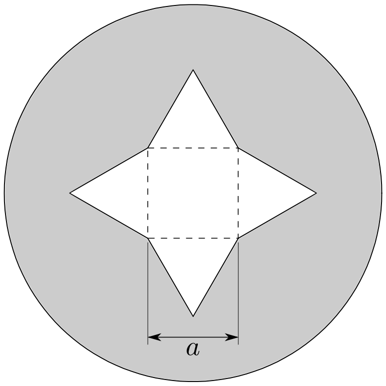  | $(1+\sqrt{3})a^2$ | $a = (0.239781)\mathbf{D}$ |
| 22 | Five-pointed star 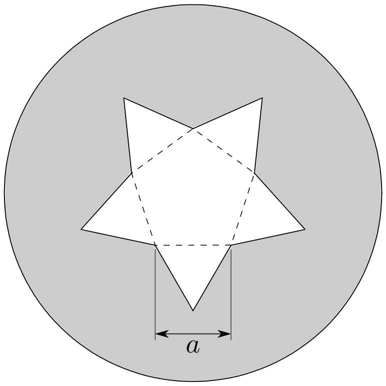  | $\frac{1}{4}\sqrt{5(5+2\sqrt{5})}a^2 + \frac{5\sqrt{3}}{4}a^2$ | $a = (0.201064)\mathbf{D}$ |
| 23 | Six-pointed star 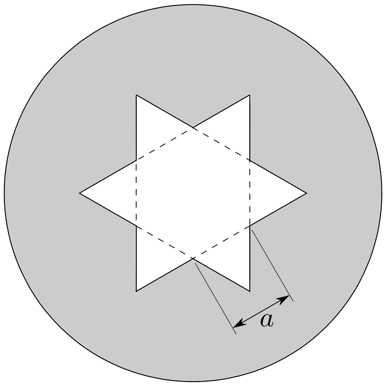  | $\frac{3\sqrt{3}}{2}a^2 + \frac{6\sqrt{3}}{4}a^2$ | $a = (0.173867)\mathbf{D}$ |

*Continued on next page*

Table S8 – Orifice geometries which were studied (*Continued from previous page*)

| **Label** | **Characteristic length of an orifice geometry** | **Area of the orifice** | **Relation with plate diameter** |
|---|---|---|---|
| 24 | Seven-pointed star 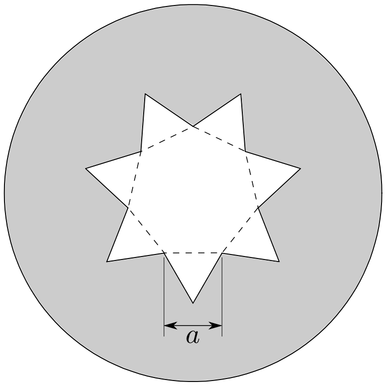  | $\frac{7}{4}a^2 \cot\left(\frac{\pi}{7}\right) + \frac{7\sqrt{3}}{4}a^2$ | $a = (0.153518)\mathbf{D}$ |
| 25 | Eight-pointed star 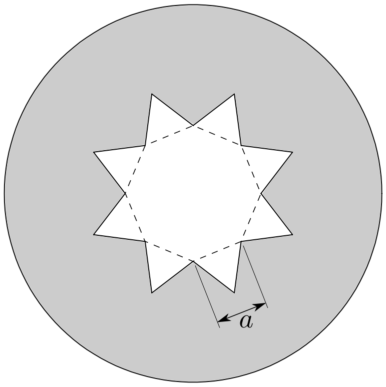  | $2\left(1+\sqrt{2}\right)a^2 + \frac{8\sqrt{3}}{4}a^2$ | $a = (0.120441)\mathbf{D}$ |

**Algorithm S1** Pseudocode of an orifice confirmation algorithm based on class binarization approach

```
function ConfirmationBlock1(orifice_id, test_data, model_library) returns a scalar
    confirmations ← 0
    models ← model_library[orifice_id]                ▷ Select models built using orifice_id
    for Model( ) in models do
        predicted_id ← Model(test_data)               ▷ Make predictions using each model
        if predicted_id = orifice_id then
            confirmations ← confirmations + 1
    return confirmations

threshold = n/2                                       ▷ n is the number of orifices

function ConfirmationAlgorithm(orifice_id, test_data, model_library, threshold) returns a message
    v ← ConfirmationBlock1(orifice_id, test_data, model_library)
    if v > threshold then
        return "Orifice confirmed."
    else
        return "Orifice not confirmed."
```

**Algorithm S2** Pseudocode of an orifice identification algorithm based on the class binarization approach. One confirmation trial is the equivalent of running the confirmation block (from algorithm S1) for a trial orifice $i$. The identified orifice corresponds to the majority vote.

```
function IdentificationBlock1(test_data, model_library) returns a vector
    V ← initialize vector of size n for confirmations
    for trial_id = 1 to n do
        V[trial_id] ← ConfirmationBlock1(trial_id, test_data, model_library)
    return V                                          ▷ Vector consisting of n orifice confirmations

function IdentificationAlgorithm1(test_data, model_library) returns orifice identity
    V ← IdentificationBlock1(test_data, model_library)
    return argmax(V)                                  ▷ Identified orifice is the orifice corresponding to majority votes
```

**Algorithm S3** Pseudocode of an orifice confirmation algorithm based on multi-class classifier approach

```
function ConfirmationBlock2(test_data, MODEL()) returns a scalar
    confirmations ← 0
    Φ ← MODEL(test_data)                         ▷ Make predictions using the multi-class classifier
    return Φ

threshold = 0.5

function ConfirmationAlgorithm2(orifice_id, test_data, threshold, MODEL()) returns a message
    Φ ← ConfirmationBlock2(test_data, MODEL())
    p ← Φ[orifice_id]                            ▷ Get the confirmation probability based on the orifice_id
    if p > threshold then
        return "Orifice confirmed."
    else
        return "Orifice not confirmed."
```

**Algorithm S4** Pseudocode of an orifice identification algorithm based on the multi-class classifier approach

```
function IdentificationAlgorithm2(test_data, MODEL()) returns orifice identity
    Φ ← MODEL(test_data)
    return argmax(Φ)                             ▷ Identified orifice is the orifice corresponding to maximum probability
```

## References

1. M Karunanethy, R Tripathi, MV Panchagnula, R Rengaswamy, User authentication system based on human exhaled breath physics. *PLOS ONE* **19**, e0301971 (2024).
2. M Christ, N Braun, J Neuffer, AW Kempa-Liehr, Time series feature extraction on basis of scalable hypothesis tests (tsfresh – a python package). *Neurocomputing* **307**, 72–77 (2018).
3. L Breiman, Random forests. *Mach. Learn.* **45**, 5–32 (2001).
4. R Andrew, R Ben, E Andrew, *Electoral System Design: The New International IDEA Handbook.* (International Institute for Democracy and Electoral Assistance), (2005).
5. F Pedregosa, et al., Scikit-learn: Machine learning in Python. *J. Mach. Learn. Res.* **12**, 2825–2830 (2011).
